# Supplementary material for: Attainable Force Approximation and Full-Pose Tracking Control of an Over-Actuated Thrust-Vectoring Modular Team UAV
Source: arXiv:2410.03445 source file (2024-10-04)
Supplement: Supplementary file 1 [file appendix01.tex]

% !TeX root = ../main.tex

\appendix{A}{Introduction}

\begin{tempsection}
\section{Introduction}
\section{Further Introduction}
\end{tempsection}
